# Supplementary material for: FLINT: A Platform for Federated Learning Integration
Source: arXiv:2302.12862 source file (2023-03-11)
Supplement: Supplementary file 1 [file appendix.tex]

%%%%%%%%%%%%%%%%%%%%%%%%%%%%%%%%%%%%%%%%%%%%%%%%%%%%%%%%%%%%%%%%%%%%%%%%%%%%%%%
%%%%%%%%%%%%%%%%%%%%%%%%%%%%%%%%%%%%%%%%%%%%%%%%%%%%%%%%%%%%%%%%%%%%%%%%%%%%%%%
% SUPPLEMENTAL CONTENT AS APPENDIX AFTER REFERENCES
%%%%%%%%%%%%%%%%%%%%%%%%%%%%%%%%%%%%%%%%%%%%%%%%%%%%%%%%%%%%%%%%%%%%%%%%%%%%%%%
%%%%%%%%%%%%%%%%%%%%%%%%%%%%%%%%%%%%%%%%%%%%%%%%%%%%%%%%%%%%%%%%%%%%%%%%%%%%%%%

\appendix
\section{SUPPLEMENTARY MATERIAL}
\section{offline async task scheduling}
\label{appendix:asyncsim}
\begin{algorithm}[H]
   \caption{An async scheduler that dispatches client tasks to workers in the correct sequence for aggregation.}
   \label{alg:asyncshedule}
\begin{algorithmic}
\STATE
   \STATE {\bfseries Input:} concurrency limit $C$
   \STATE initialize $minQueue$ as min priority queue
   \STATE $c \gets 0$ (concurrency)
   \STATE $time \gets 0$ (virtual clock)
  
   \STATE \textbf{function} $createTask()$
      \STATE\hskip1.0em $task \gets sampleNextClient(time)$
       \STATE\hskip1.0em $minQueue.insert(task.startTime, task, START)$
       \STATE\hskip1.0em $minQueue.insert(task.endTime, task, END)$
   \STATE \textbf{end function}

   \STATE $createTask()$
   \REPEAT
   \STATE $task, flag \gets minQueue.pop()$
   \IF{$flag$ is $START$}
   \STATE $c \gets c + 1$
   \STATE $createTask()$
   \ELSE
   \STATE $c \gets c - 1$
   \IF{$c = C - 1$}
   \STATE $createTask()$
   \ENDIF
   \STATE $dispatchTaskToWorker(task.client)$
   \STATE $time \gets task.endTime$
   \ENDIF
   \UNTIL{$time > duration$}
\end{algorithmic}
\end{algorithm}

\section{Applying the Decision Framework}

\appendix
%%%%%%%%%%%%%%%%%%%%%%%%%%%%%%%%%%%%%%%%%%%%%%%%%%%%%%%%%%%%%%%%%%%%%%%%%%%%%%%
%%%%%%%%%%%%%%%%%%%%%%%%%%%%%%%%%%%%%%%%%%%%%%%%%%%%%%%%%%%%%%%%%%%%%%%%%%%%%%%
